# Supplementary material for: Constraints on low-mass, relic dark matter candidates from a surface-operated SuperCDMS single-charge sensitive detector
Source: arXiv:2005.14067 ancillary file (2021-01-29)
Supplement: Supplementary file 1 [file HVeV_Run_2_Data_Release.pdf]

# HVeV Run 2 Data Release

SuperCDMS Collaboration

January 28, 2021

This document accompanies the public release of data from the second run of the SuperCDMS quantization-sensitive detector known as HVeV Run 2. This release includes all experimental data necessary to reproduce the dark matter (DM) search results in <https://journals.aps.org/prd/abstract/10.1103/PhysRevD.102.091101> [1]. The provided data and information allows the community to use these data for their own analyses or for reproducing the HVeV Run 2 results. Questions about this release should be directed to [supercdms\\_publications@lists.astro.caltech.edu](mailto:supercdms_publications@lists.astro.caltech.edu).

The provided experimental and supplemental data files and information are described in Sec. 1. Due to the discrete nature of the ionization signal in the HVeV detector, the continuous DM electron recoil spectrum has to be convolved with an ionization model that depends on the Fano factor  $F$ , described in Sec. 2. The probed DM models and the conversion of the final spectrum into the physics limits are described in Sec. 3. The published upper limits on light DM-electron scattering, dark photon absorption, and axion-like particle (ALP) absorption are computed based on Poissonian statistics. The background is assumed to be completely unknown for this analysis; in other words, all events are treated as potential signals in order to set conservative limits.

## 1 Description of the Files

Twenty-six tab-separated value files (.tsv) are included in this data release and can be found in various folders of the accompanying .zip file. The names and descriptions of these files are provided in this section.

### 1.1 HVeV data

#### 1.1.1 Energy Spectrum

The data release contains two spectral data files:

- `HVeVR2data/dm_100V_final_DatQua_191230.tsv` (Fig. 1),
- `HVeVR2data/laser_100V_final_DatQua_191230.tsv` (Fig. 1).

The file names indicate whether the dataset is for the DM-search (`dm`) or the laser-calibration (`laser`). The data in these files have had all the cuts described in Ref. [1] applied to obtain the data quality needed for limit-setting. The data within are plotted in Fig. 1.

Each of these files contains a single column of ASCII numbers written in scientific format followed by a newline symbol,

```
1.012345678901234567e+01
2.012345678901234567e+02
3.012345678901234567e+03
.....
```

Readers should be able to open them in any common text reader or import them to their scripts. For example, in Python:

```
numpy.loadtxt("HVeVR2data/laser_100V_final_DatQua_191230.tsv")
```

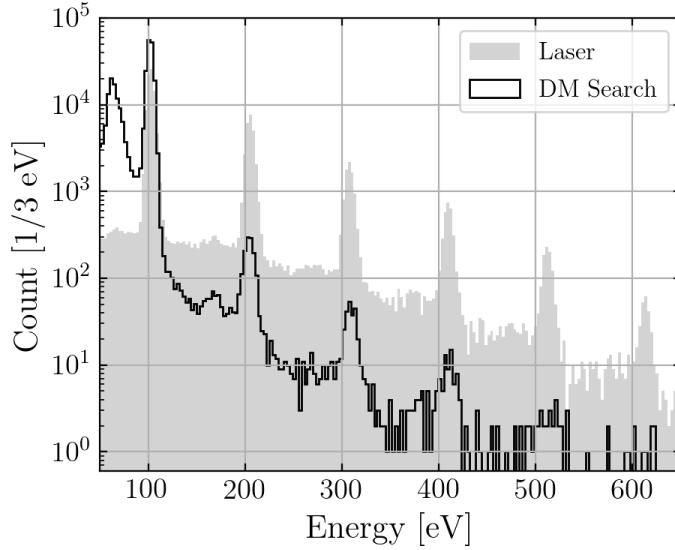

Figure 1: The DM-search (line) and laser-calibration (shaded) spectra. The data are binned by 3 eV and plotted for the analysis region of interest, 50 eV to 650 eV.

Each of the numbers represents one recorded energy from an event that passed all the cuts, calibrated to the unit of eV using the laser-calibration data as described in Ref. [1].

### 1.1.2 Efficiency

The data release contains the cut efficiency file:

- HVeVR2data/efficiency\_100V\_final\_Fit\_191230.tsv (Fig. 2).

The data file is for the fitted efficiency curve, as opposed to the binned efficiencies calculated from the laser data. Readers may find the details about the efficiency curve in Ref. [1].

The file contains four columns of numbers in the same format used by the spectral data (see 1.1.1), with tab symbols separating the numbers in each row, e.g.

|                 |                  |                  |                  |
|-----------------|------------------|------------------|------------------|
| 7.000000000e+01 | 7.2387100085e-01 | 8.0446868488e-01 | 8.8506636892e-01 |
| 7.050000000e+01 | 7.2571194961e-01 | 8.0658277731e-01 | 8.8745360502e-01 |
| 7.100000000e+01 | 7.2813933384e-01 | 8.0866765164e-01 | 8.8919596944e-01 |

.....

Again, the readers may open it in text readers or import the data by (Python)

```
numpy.loadtxt("HVeVR2data/efficiency_100V_final_Fit_191230.tsv", delimiter="\t")
```

The numbers in the first column represent the energies in eV which are evenly spaced by 0.5 eV. The second, third, and fourth columns, respectively, are the lower bound, central value, and higher bound for the corresponding cut efficiency at each energy, normalized and bounded by 1. Fig. 2 shows the attached efficiency curve with the uncertainty band.

## 1.2 Supplementary Data: Complex Conductivity and Photoelectric Absorption Cross Section

The files described in this section do not contain SuperCDMS data. They contain external data of the complex conductivity  $\tilde{\sigma}$  and the photoelectric absorption cross section  $\sigma_{\text{p.e.}}$ . The complex conductivity is

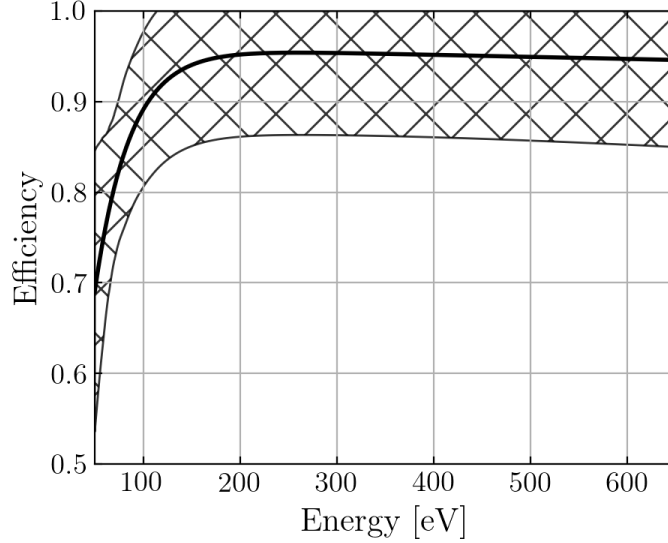

Figure 2: The fitted efficiency curve. The solid curve represents the central value of the fit, while the hatched region represents its uncertainty.

necessary to calculate the published dark photon kinetic mixing limit, whereas the photoelectric absorption cross section is necessary to calculate the published ALP-electron coupling constant limit. For more information on dark photon absorption and ALP absorption see Secs. 3.2.2 and 3.2.3, respectively. The photoelectric cross section, as well as the real and imaginary parts of  $\tilde{\sigma} = \sigma_1 + i\sigma_2$ , are included in separate files, described in more detail in this section.

### 1.2.1 Real Part of the Complex Conductivity and Photoelectric Absorption Cross Section

The photoelectric cross section and the real part of the complex conductivity are proportional to each another by  $\sigma_1 = n\sigma_{\text{p.e.}}$ , where  $n$  is the energy-dependent index of refraction for Si. The  $\sigma_1$  information is provided in units of conductivity (eV), and the  $\sigma_{\text{p.e.}}$  information is provided in units of an absorption coefficient ( $\text{cm}^2/\text{g}$ ). These units follow the notation in Eqs. 23 and 26, and were used to calculate the final results. The six photoelectric cross section data files listed below are included in this data release. The first column in these data files corresponds to the photon energies in units of keV. The second column corresponds to either  $\sigma_1$  in units of eV or  $\sigma_{\text{p.e.}}$  in units of  $\text{cm}^2/\text{g}$  as indicated in the file names (`pexsec...<column-1 units>_<column-2 units>_interp.tsv`):

- `SupplData/pexsec_Si_lower_keV_eV_interp.tsv` (Fig. 3 Top),
- `SupplData/pexsec_Si_nominal_keV_eV_interp.tsv` (Fig. 3 Top),
- `SupplData/pexsec_Si_upper_keV_eV_interp.tsv` (Fig. 3 Top),
- `SupplData/pexsec_Si_lower_keV_cm2g_interp.tsv` (Fig. 3 Bottom),
- `SupplData/pexsec_Si_nominal_keV_cm2g_interp.tsv` (Fig. 3 Bottom),
- `SupplData/pexsec_Si_upper_keV_cm2g_interp.tsv` (Fig. 3 Bottom).

The data provided in the files are linearly interpolated data points based on measurements found in literature and the methodology described in Ref. [1] and here. Readers can import these files and interpolate the data to compute the dark photon absorption rate or ALP absorption rate at any mass in this energy range. Three versions of  $\sigma_1$  and  $\sigma_{\text{p.e.}}$  are included in the data release. One is referred to as “nominal data”,

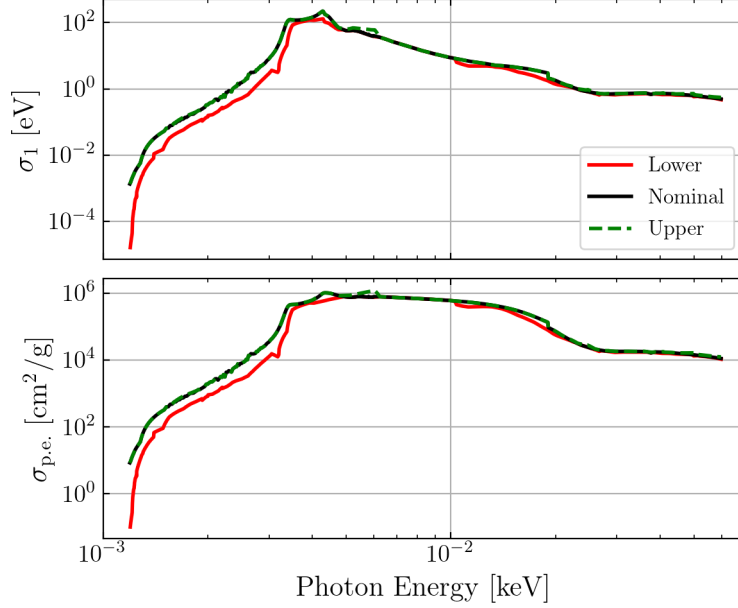

Figure 3: Real part of the complex conductivity  $\sigma_1 = \text{Re}(\tilde{\sigma})$  (top) and photoelectric absorption cross section  $\sigma_{\text{p.e.}} = \frac{1}{n}\sigma_1$  (bottom) for Si. The black curve is the nominal data from Ref [2]. The red and green curves are the lower and upper  $\sigma_1$  and  $\sigma_{\text{p.e.}}$  curves, respectively, determined by tracing upper and lower bounds of the published data from the literature search after applying temperature corrections.

which is the  $\sigma_1/\sigma_{\text{p.e.}}$  data that is commonly used in dark absorption searches by other collaborations and scientists (for example in Hochberg et al. [2]). The others are referred to as the “upper” and “lower” curves, which represent the highest and lowest reasonable cross section, accounting for discrepancies in the literature as well as temperature dependencies. To generate the upper and lower curves, a temperature correction is applied to the published data from the literature search (see Ref [1]). The temperature correction accounts for the temperature dependence of indirect, phonon-assisted absorption that occurs at energies below the direct band gap ( $\sim 3$  eV), well within the energy region accessible by the HVeV detector. We followed the methodology and analytical model for photon absorption found in Ref. [3] to extrapolate the published data below 4 eV to a temperature of 50 mK. The upper and lower curves are derived by tracing upper and lower bounds of the data after the temperature correction is applied. To ensure that the upper and lower curves are always the highest and lowest values of  $\sigma_1$  or  $\sigma_{\text{p.e.}}$  used in the analysis, the nominal curve data (which did not have the temperature correction applied) are also included when tracing the upper and lower bounds. The nominal, upper, and lower  $\sigma_1$  and  $\sigma_{\text{p.e.}}$  curves are shown in Fig. 3.

### 1.2.2 Imaginary Part of the Complex Conductivity: Phase Lag of the System

The imaginary value of the conductivity  $\sigma_2$  can be interpreted as the delay of the charge carrier response to quick changes in the electric field. This value depends on the energy of the incoming photon, or, in the context of dark photon searches, on the energy of the incoming dark photon. In the case of  $\sigma_2$ , there is much less literature that allows for a similarly detailed study as with  $\sigma_1$ . For this reason, only one set of  $\sigma_2$  values was used for the limit calculation. These values are from Ref [2] and are included in this data release in the following file:

- SupplData/Conductivity\_Si\_keV.eV\_Imaginary.tsv (Fig. 4).

The first column in this data file contains the photon energy in units of keV, and the second column contains the corresponding  $\sigma_2$  values in units of eV. The absolute values of  $\sigma_2$  are shown in Fig. 4.

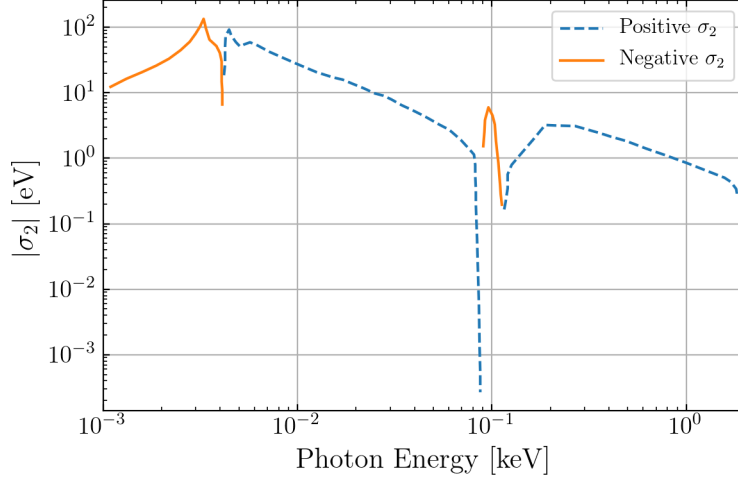

Figure 4: Imaginary part of the complex conductivity  $\sigma_2 = \text{Im}(\tilde{\sigma})$  for Si. The blue-dashed (orange-solid) curve are positive (negative) values of  $\sigma_2$  from Ref [2].

### 1.3 Exclusion limits

The files containing the four published exclusion limits from Ref [1], including the bands that represent our estimate of the systematic uncertainty, are described in this section. The respective limits are shown in Fig. 5. For each limit, one file is included in this data release:

- `limits/HVeV_Run2_DMe_F1_100V_Limit.tsv` (Fig. 5a),
- `limits/HVeV_Run2_DMe_Fq2_100V_Limit.tsv` (Fig. 5b),
- `limits/HVeV_Run2_DPA_100V_Limit.tsv` (Fig. 5c),
- `limits/HVeV_Run2_ALP_100V_Limit.tsv` (Fig. 5d).

The first two files contain the scattering cross section limit for DM scattering off electrons for two different DM form factors:  $F_{\text{DM}} = 1$  and  $F_{\text{DM}} \propto q^{-2}$ , where  $q$  is the momentum transfer. The form factor is indicated in the file name as “F1” and “Fq2”, respectively. The third and fourth files contain the limits on dark photon kinetic mixing and the axioelectric coupling constant, respectively. All files consist of four columns:

- Column 1: DM mass in  $\text{MeV}/c^2$  for DM-e scattering and in  $\text{keV}/c^2$  for dark photon absorption and axion-like particle absorption.
- Column 2: reported limit.
- Column 3: lower bound of limit band.
- Column 4: upper bound of limit band.

The limit bands represent our estimates of the systematic uncertainty. The limit and propagated uncertainty was computed separately for each assumption of the Fano factor in the ionization model (see Secs. 3.3 and 2.1). The limit bands that are shown in Fig. 5 envelop the upper and lower uncertainties (the  $\pm 1\sigma$  values) of all three limits obtained using the different Fano factor assumptions. At most masses, the uncertainty bands are dominated by the varying Fano factor assumption (see Sec. 2.1); the exception is for  $\lesssim 4 \text{ eV}/c^2$  in the dark photon and ALP absorption models, where the uncertainty is dominated by the discrepancy in the photoelectric absorption cross section (see Sec. 1.2.1). The reported limit in each file is the limit computed with a Fano factor of 0.155.

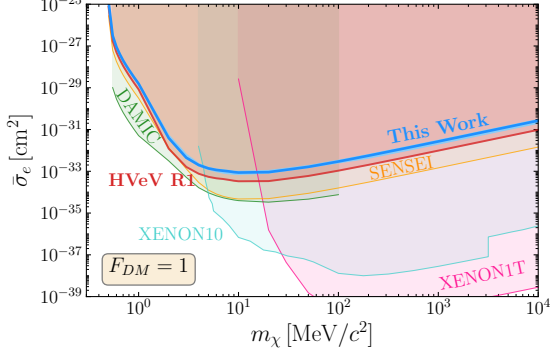

(a) HVeV Run 2 limit (blue) on the DM-electron scattering cross section  $\bar{\sigma}_e$  for DM interacting with electrons via a heavy mediator ( $F_{DM} = 1$ ) compared to the results from SuperCDMS HVeV Run 1 [4], DAMIC [5], SENSEI [6], XENON10 [7, 8], and XENON1T [9].

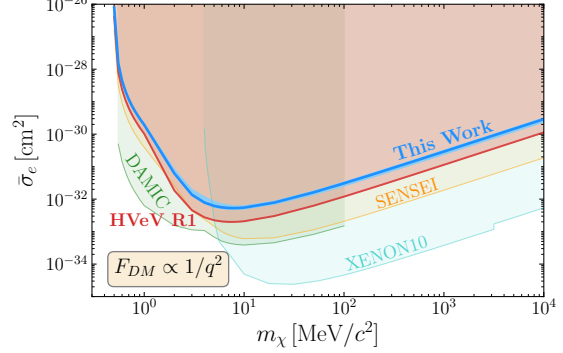

(b) HVeV Run 2 limit (blue) on the DM-electron scattering cross section  $\bar{\sigma}_e$  for DM interacting with electrons via an ultra-light mediator ( $F_{DM} \propto 1/q^2$ ) compared to the results from SuperCDMS HVeV Run 1 [4], DAMIC [5], SENSEI [6], and XENON10 [7, 8].

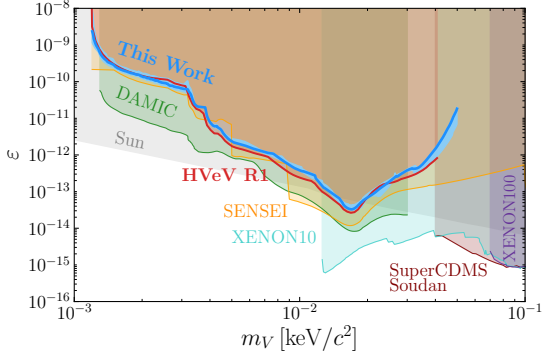

(c) HVeV Run 2 limit (blue) on the dark photon kinetic mixing parameter  $\epsilon$  compared to the results from SuperCDMS HVeV Run 1 [4], DAMIC [5], SENSEI [6], XENON10, XENON100 [10], and SuperCDMS Soudan [11]. Exclusion from anomalous energy loss mechanisms in the Sun is also shown [12].

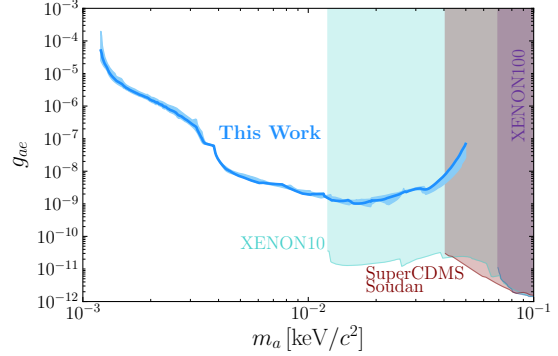

(d) HVeV Run 2 limit (blue) on the axioelectric coupling constant  $g_{ae}$  compared to the results from XENON10, XENON100 [10], and SuperCDMS Soudan [11]. The entire region shown is disfavoured by the observed cooling of red giant and white dwarf stars [13, 14, 15].

Figure 5: HVeV Run 2 DM search limits as published in Ref [1]. The blue lines are the reported limits with a Fano factor of 0.155. The light blue bands represent our estimate of the systematic uncertainty, which are dominated by varying the Fano factor assumption in the ionization model from  $F = 10^{-4}$  to 0.3. The exception is for dark photon and ALP masses  $\lesssim 4 \times 10^{-3}$  keV/ $c^2$ , where the uncertainty is dominated by the discrepancy in the photoelectric absorption cross section.

## 2 Detector Response Model

To compute the detector response to a given energy deposition from any DM model, we need to model the number of  $e^-h^+$  pairs  $n_{\text{eh}}$  produced for a given energy deposited in the crystal. Furthermore, the analysis performed in Ref. [1] incorporated charge trapping and impact ionization into the detector response model. Finally, the detector response models are converted from an ionization energy scale in units of  $n_{\text{eh}}$  to an eV energy scale. This section provides the details necessary to replicate the detector response model used for this analysis.

### 2.1 Ionization Production

The mean number of  $e^-h^+$  pairs produced by an electron recoil of energy  $E_\gamma$  is given by the piece-wise function

$$\langle n_{\text{eh}}(E_\gamma) \rangle = \begin{cases} 0 & E_\gamma < \epsilon_{\text{gap}} \\ 1 & \epsilon_{\text{gap}} < E_\gamma < \epsilon_{\text{eh}} \\ E_\gamma/\epsilon_{\text{eh}} & \epsilon_{\text{eh}} < E_\gamma \end{cases} \quad (1)$$

where  $\epsilon_{\text{gap}} = 1.2$  eV and  $\epsilon_{\text{eh}} = 3.8$  eV [16]. The probability distributions in the first two cases are delta functions, necessary in order to conserve energy. In the third case, discrete distributions are generated with an arbitrary Fano factor  $F$  defined as

$$F = \frac{\sigma^2}{\mu} \quad (2)$$

where  $\mu = \langle n_{\text{eh}} \rangle$  is the mean of the distribution, and  $\sigma^2$  is the variance. A completely uncorrelated (Poisson) process has a Fano factor of 1, but in most radiation detectors Fano factors on the order of 0.1-0.2 are found due to the fact that large deviations from the mean are kinematically suppressed.

Probability distributions for a given mean number of  $e^-h^+$  pairs and Fano factor were generated using a binomial distribution with  $n$  trials of probability  $p$ . In other words, the selected values of  $F$  and  $\mu$  are used to determine the  $n$  and  $p$  values of the binomial distribution and hence the probability distribution of  $e^-h^+$ -pair production. The binomial distribution has variance  $\sigma^2$  and mean  $\mu$  that obey the relations

$$\mu = np \quad (3)$$

$$\sigma^2 = np(1-p) = \mu(1-p) \quad (4)$$

The  $n$  and  $p$  values can then be calculated from the Fano factor and mean number of  $e^-h^+$  pairs as

$$F = \frac{\sigma^2}{\mu} = (1-p) \rightarrow p = 1-F \quad (5)$$

$$n = \frac{\mu}{p} = \frac{\mu}{1-F} \quad (6)$$

The caveat to these equations is that the binomial distribution is quantized, and thus  $n$  is an integer; this means that we have to interpolate between the distributions for the integers directly above and below the fractional mean value given by the mean and Fano factor combination. This is done by setting an upper and lower bound on the number of  $e^-h^+$  pairs ( $n_l$  and  $n_h$ ) and converting that to an upper and lower bound on the Fano factor ( $F_l$  and  $F_h$ ), using the equations below:

$$n_l(\mu, F) = \text{floor} \left( \frac{\mu}{1-F} \right) \quad (7)$$

$$n_h(\mu, F) = \text{ceil} \left( \frac{\mu}{1-F} \right) \quad (8)$$

$$F_l(\mu, F) = 1 - \mu/n_l(\mu, F) \quad (9)$$

$$F_h(\mu, F) = 1 - \mu/n_h(\mu, F) \quad (10)$$

Using  $F_l$  and  $F_h$ , upper and lower binomial distributions ( $P_l$  and  $P_h$ ) can be constructed. The final probability distribution  $P(x|\mu, F)$  is found by interpolating between  $P_l$  and  $P_h$ , as outlined below:

$$\Delta F(\mu, F) = \frac{F - F_l(\mu, F)}{F_h(\mu, F) - F_l(\mu, F)} \quad (11)$$

$$P_l(x|\mu, F) = \text{Binomial}(x|n_l(\mu, F), 1 - F_l(\mu, F)) \quad (12)$$

$$P_h(x|\mu, F) = \text{Binomial}(x|n_h(\mu, F), 1 - F_h(\mu, F)) \quad (13)$$

$$P(x|\mu, F) = P_l(x|\mu, F)(1 - \Delta F(\mu, F)) + P_h(x|\mu, F)\Delta F(\mu, F) \quad (14)$$

$P(x|\mu, F)$  is the weighted mean of two binomial distributions given a non-integer mean, with weights defined by how close the Fano factor of the binomial distribution is to the intended Fano factor.

The limits in Ref [1] and their propagated uncertainty are calculated separately using three different values for the Fano factor: the value measured at high energy,  $F = 0.155$ , and the values of  $F = 10^{-4}$  and  $F = 0.3$  that are assumed to cover the systematic uncertainty of the Fano factor at the low-energy regime where this analysis is relevant [17]. As mentioned in Sec.1.3, the Fano factor was the dominant source of uncertainty in the exclusion limits except for the low mass dark photon and ALP regions.

## 2.2 Charge Trapping and Impact Ionization

The detector response uses a simplistic model to account for the effects of charge trapping (CT) and impact ionization (II). Charge trapping occurs when a propagating electron or hole falls into a charge vacancy in the crystal, reducing the total number of electrons or holes that traverse the entire detector and lowering the measured event energy. Impact ionization occurs when an electron or hole liberates an additional loosely bound charge in the crystal, thereby increasing the measured energy for an event.

CT and II in the detector is described by a two-parameter model, whose inputs are the fractional probabilities of CT  $f_{\text{CT}}$  and II  $f_{\text{II}}$ . The model assumes the probability of a CT or II process occurring for a single charge is a flat distribution across the thicknesses of the detector, and that the probabilities are consistent between electrons and holes. Finally, this model only accounts for first-order processes (i.e. CT or II after a prior II occurred is not considered) because the probability of higher-order processes are sub-percentage. The probability distribution function  $P$  as a function of energy  $E$  (in units of  $n_{\text{eh}}$ ) and the fractional probability of CT and II up to  $N$   $e^-h^+$  pairs is given by:

$$P(E, f_{\text{CT}}, f_{\text{II}}) = \sum_{n_{\text{eh}}=1}^N P_1(n_{\text{eh}}|\mu, F) \sum_{n_{\text{CT}}=0}^{n_{\text{eh}}} \sum_{n_{\text{II}}=0}^{n_{\text{eh}}-n_{\text{CT}}} P_f(f_{\text{CT}}, f_{\text{II}}) p(E, n_{\text{eh}}, n_{\text{CT}}, n_{\text{II}}), \quad (15)$$

where  $P_1(n_{\text{eh}}|\mu, F)$  is the probability of  $n_{\text{eh}}$   $e^-h^+$  pairs for a given Fano factor and mean number of  $e^-h^+$  pairs determined by the ionization production model (see Sec. 2.1).  $n_{\text{CT}}$  and  $n_{\text{II}}$  are the number of  $e^-h^+$  pairs with an occurrence of CT and II, respectively, where  $n_{\text{CT}} + n_{\text{II}} \leq n_{\text{eh}}$ . The term  $p(E, n_{\text{CT}}, n_{\text{II}}, n_{\text{eh}})$  describes the PDF shape as a function of  $E$  for a given  $n_{\text{CT}}$  and  $n_{\text{II}}$ , and is given by:

$$p(E, n_{\text{eh}}, n_{\text{CT}}, n_{\text{II}}) = \begin{cases} \frac{1}{\sigma_E \sqrt{2\pi}} \exp \left[ -\frac{1}{2} \left( \frac{E - n_{\text{eh}}}{\sigma_E} \right)^2 \right] & n_k = 0 \\ \left[ \frac{1}{2(n_k - 1)!} \sum_{l=0}^{n_k} (-1)^l \binom{n_k}{l} (u(E) - l)^{n_k - 1} \text{sgn}(u(E) - l) \right] * G(\sigma_E) & n_k \geq 1, \end{cases} \quad (16)$$

where  $n_k = n_{\text{CT}} + n_{\text{II}}$ ,  $u(E) = E - n_{\text{eh}} + n_{\text{CT}}$ , and  $\sigma_E$  is the detector energy resolution. This analysis used the weighted average energy resolution of  $\sigma_E = \sigma_{\langle E \rangle} = 3.6 \text{ eV}$  [1]. In the case where no  $e^-h^+$  pairs have charge trapping or impact ionization ( $n_k = 0$ ),  $p(E, n_{\text{eh}}, n_{\text{CT}}, n_{\text{II}})$  describes a Gaussian distribution centered around  $n_{\text{eh}}$ . In the case where at least one  $e^-h^+$  pair has charge trapping or impact ionization ( $n_k \geq 1$ ),  $p(E, n_{\text{eh}}, n_{\text{CT}}, n_{\text{II}})$  describes the uniform sum distribution convolved with a Gaussian distribution  $G(\sigma_E)$  representing the detector energy resolution. The term  $u(E)$  places each PDF in the correct location in energy for a given number of  $e^-h^+$  pairs.

Lastly, the term  $P_f(f_{\text{CT}}, f_{\text{II}})$  in Eq. 15 describes the probability of  $n_{\text{CT}}$  and  $n_{\text{II}}$  occurring given the

fractional probabilities  $f_{\text{CT}}$  and  $f_{\text{II}}$ :

$$P_f(f_{\text{CT}}, f_{\text{II}}) = \frac{n_{\text{eh}}!}{n_{\text{CT}}!n_{\text{II}}!(n_{\text{eh}} - n_{\text{CT}} - n_{\text{II}})!} (\kappa\gamma)^{n_{\text{eh}} - n_{\text{CT}} - n_{\text{II}}} (\gamma(1 - \kappa))^{n_{\text{CT}}} (1 - \gamma)^{n_{\text{II}}} \quad (17)$$

$$\gamma = 1 - f_{\text{II}} \quad (18)$$

$$\kappa = \frac{f_{\text{CT}} + f_{\text{II}} - 1}{f_{\text{II}} - 1}. \quad (19)$$

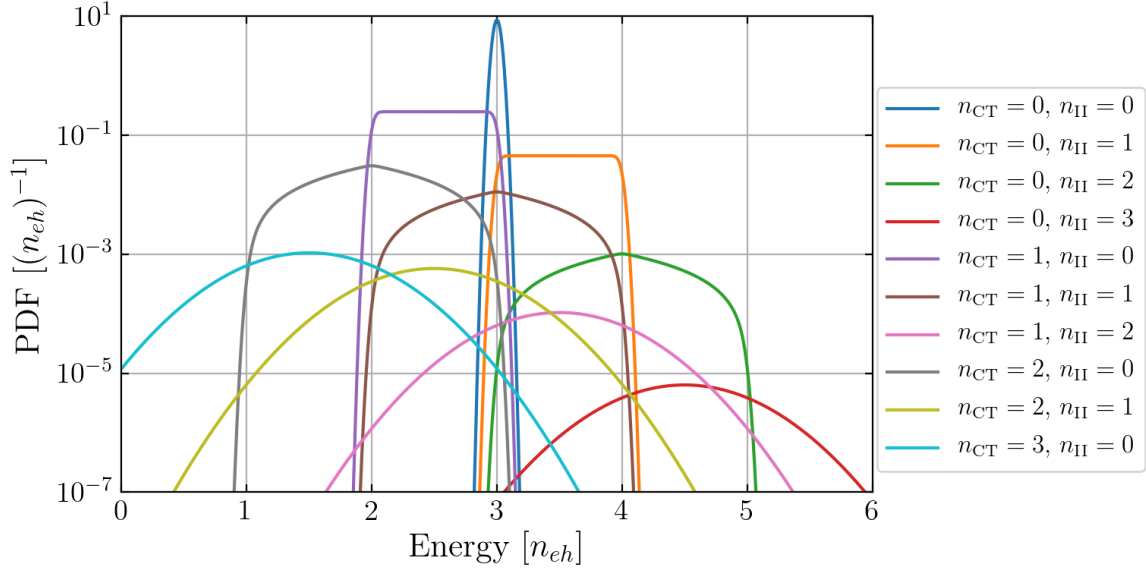

Figure 6: Example of the charge trapping (CT) and impact ionization (II) probability distribution model with  $n_{\text{eh}} = 3$  and fractional probabilities  $f_{\text{CT}} = 0.11$ , and  $f_{\text{II}} = 0.02$ . Each curve describes the probability distribution for a given number of  $e^-h^+$  pairs that have an occurrence of charge trapping ( $n_{\text{CT}}$ ) and/or impact ionization ( $n_{\text{II}}$ ), following Eqs. 16 and 17. This example uses a detector energy resolution of  $\sigma_E = 0.03 n_{\text{eh}}$ .

An example of the charge trapping and impact ionization model is shown in Fig. 6 with  $n_{\text{eh}} = 3$ ,  $f_{\text{CT}} = 0.11$ , and  $f_{\text{II}} = 0.02$ . Additionally, a slightly modified version of this model was fit to the laser calibration data to determine the values of  $f_{\text{CT}}$  and  $f_{\text{II}}$ . The model used for the laser calibration data is identical to the description above, except the  $P_1(n_{\text{eh}}|\mu, F)$  term in Eq. 15 is replaced with a Poisson distribution, i.e.

$$P_1(n_{\text{eh}}|\mu, F) \rightarrow P_{\text{Poisson}}(n_{\text{eh}}, \lambda), \quad (20)$$

where  $\lambda$  is the mean number of photons per laser pulse.

### 2.3 Conversion to eV Scale

Sections 2.1 and 2.2 describe the response caused by  $e^-h^+$  pair ionization produced by particle interactions within the detector and the probability density functions of  $n_{\text{eh}}$ . However, the total phonon energy measured by the detector,  $E_{ph}$ , is the recoil/absorption energy of the scattering/absorbed particle,  $E_r$ , plus the energy gained via ionization production and Neganov-Trofimov-Luke phonon amplification:

$$E_{ph} = E_r + n_{\text{eh}} \cdot e \cdot V_{\text{bias}}, \quad (21)$$

where  $e$  is the absolute value of the electron charge. The final detector response model is determined by scaling the energies of the ionization production model by  $V_{\text{bias}}$  (thereby converting it to an eV energy scale) and then adding the  $E_r$  energy component to them. To keep the proper normalization of the ionization production model, the probability densities are subsequently scaled by  $1/V_{\text{bias}}$ .

### 3 Limit Calculation

In order to compute DM search limits, three main inputs are needed: the experimental spectrum, the DM model to be probed, and a limit setting technique. This section will describe each of these pieces, which together resulted in the published HVeV Run 2 DM search limits shown in Sec. 1.3 and their corresponding uncertainties.

#### 3.1 Experimental Input

The HVeV Run 2 experimental inputs are the observed energy spectrum (Fig. 1, Sec. 1.1.1), the signal efficiency (Fig. 2, Sec. 1.1.2), the analysis thresholds (both an upper and lower threshold), and the total exposure. The lower analysis threshold is 50 eV, and the upper threshold is 650 eV. The total exposure after all livetime cuts were applied is 1.2 gram-days. The detector energy resolution  $\sigma_{\langle E \rangle} = 3.6$  eV is determined by averaging over the resolutions of the first six Gaussian-fitted  $e^-h^+$ -pair peaks from the combined laser-calibration data, weighted by the corresponding uncertainty in each peak. Finally, the charge trapping and impact ionization probabilities measured from the laser-calibration data are 11 % and 2 %, respectively. No further experimental information related to the HVeV detector is necessary to calculate limits for the DM models presented in Ref [1].

#### 3.2 Dark Matter Models

Four DM models were probed in Ref [1]: light DM interacting with electrons via a heavy dark photon mediator, light DM interacting with electrons via an ultra-light dark photon mediator, dark photon absorption via the kinetic mixing with the Standard Model (SM) photon, and ALP absorption via the axioelectric effect. Each DM candidate was assumed to constitute all relic DM in the universe. The first two models and their event rate calculations are outlined in Sec. 3.2.1. The third and fourth models and their event rate calculations are outlined in Secs. 3.2.2 and 3.2.3, respectively.

##### 3.2.1 Light DM - Electron Scattering

The scattering rate of light DM with electrons is given by the equation

$$\frac{dR}{d \ln E_R} = V_{\text{det}} \frac{\rho_{\text{DM}}}{m_{\text{DM}}} \frac{\rho_{\text{Si}}}{2m_{\text{Si}}} \bar{\sigma}_e \alpha \frac{m_e^2}{\mu_{\text{DM},e}^2} I_{\text{crystal}}(E_e; F_{\text{DM}}), \quad (22)$$

where  $V_{\text{det}} = 1 \times 1 \times 0.4 \text{ cm}^3$  is the detector volume;  $\rho_{\text{DM}}$  is the relic DM density (assuming  $\rho_{\text{DM}} \approx 0.3 \text{ GeV/cm}^3$ );  $m_{\text{DM}}$  is the DM mass;  $\rho_{\text{Si}} = 2.33 \text{ g/cm}^3$  and  $m_{\text{Si}} = 28.09 \text{ amu}$  are the silicon density and mass;  $\bar{\sigma}_e$  is the DM-e scattering cross section;  $\mu_{\text{DM},e}$  is the reduced mass of the DM electron system;  $I_{\text{crystal}}$  is the crystal form factor;  $E_e$  is the electron energy; and  $F_{\text{DM}}$  is the DM form factor.

Two common benchmark models were used to calculate the limits shown in Figs. 5a and 5b. The first is a model with  $F_{\text{DM}} = 1$ , assuming DM interacts with electrons via a heavy dark photon mediator. The second is a model with  $F_{\text{DM}} = \alpha^2 m_e^2 / q^2$ , assuming the DM-electron interaction is mediated by an ultra-light dark photon.

The differential rate calculation in Eq. 22 is further dependent on  $I_{\text{crystal}}$ , and thus requires knowledge of the electronic structure of the target crystal. The rate calculation including the integration of  $I_{\text{crystal}}$ , is provided by the QEdark tool<sup>1</sup>. The published calculations describe the yield for electron recoils up to 50 eV, both as continuous (in units of deposited energy) and as quantized (in  $e^-h^+$  pairs) differential rates. For Ref [1], the continuous rates are used, and are quantized using our own, more sophisticated quantization model (see Sec. 2) that is convolved with the detector resolution  $\sigma_{\langle E \rangle}$  and incorporates charge trapping (CT) and impact ionization (II).

<sup>1</sup>Information on the QEdark calculation as well as the calculated rates for silicon are publicly available at <http://ddlDM.physics.sunysb.edu/ddlDM/>.

### 3.2.2 Dark Photon Absorption

The probed dark photon model assumes kinetic mixing between the dark photon and the SM photon. The predicted event rate for dark photon absorption is given by

$$R = V_{\text{det}} \frac{\rho_{\text{DM}}}{m_V} \varepsilon_{\text{eff}}^2 (m_V, \tilde{\sigma}) \sigma_1(m_V c^2), \quad (23)$$

where  $m_V$  is the dark photon mass and  $\varepsilon_{\text{eff}}$  is the effective kinetic mixing angle.  $\varepsilon_{\text{eff}}$  is directly related to the parameter of interest, the kinetic mixing parameter  $\varepsilon$ :

$$\varepsilon_{\text{eff}}^2 = \varepsilon^2 \cdot \frac{m_V^4}{[m_V^2 - \text{Re}\Pi]^2 + [\text{Im}\Pi]^2}. \quad (24)$$

$\Pi$  is the polarization tensor,

$$\Pi(E = m_V c^2) \approx -i \cdot \tilde{\sigma} \cdot m_V c^2, \quad (25)$$

which can be substantially altered by in-medium effects [18]. For  $m_V \gtrsim 100 \text{ eV}/c^2$ ,  $\varepsilon$  is well-approximated by  $\varepsilon_{\text{eff}}$ . For smaller dark photon masses, as considered in Ref. [1], in-medium corrections can no longer be neglected, and Eq. 24 must be used. Both Eq. 23 and Eq. 24 require knowledge of  $\sigma_1 = \text{Re}(\tilde{\sigma})$ , the photoelectric cross section (see Fig. 3 and Sec. 1.2.1). Equation 24 further requires knowledge of  $\sigma_2 = \text{Im}(\tilde{\sigma})$  (see Fig. 4 and Sec. 1.2.2).

The dark photon spectrum in the continuous regime resulting from Eq. 23 consists of a sharp line at the electron recoil energy corresponding to the dark photon mass, broadened by the energy resolution of the detector. To calculate the dark photon signal spectrum in the quantized regime, the ionization model described in Sec. 2 is employed, and the quantized spectrum is again convolved with  $\sigma_{\langle E \rangle}$  with CT and II accounted for (see Sec. 2.2). Furthermore, the in-medium correction is accounted for in the signal rate model calculation by substituting Eq. 24 into Eq. 23. By doing so, the resulting limit is set directly on the parameter of interest,  $\varepsilon$ .

### 3.2.3 Axion-Like Particle Absorption

The axion is a hypothetical particle theorized to solve the strong CP problem in QCD [19], which may also serve as the dominant component of the dark matter. The typical mass of the QCD axion is predominantly constrained by its coupling to the QCD kinetic term  $G_{\mu\nu}^a G^{a\mu\nu}$  and ranges from  $(10^{-5} - 10^{-3}) \text{ eV}/c^2$  [20]. This experiment is not sensitive to this dark matter mass range and thus is not sensitive to the QCD axion. However, any axion model allows for derivative-type couplings between the axion and the axial currents of quarks and photons [21]. For an interaction of this form, a bound electron may absorb the energy of the axion and be ejected from its atom through a phenomenon called the axioelectric effect, which is an analogue to the photoelectric effect between photons and electrons. Axion-like particles (ALPs) have this axioelectric effect but do not solve the strong CP problem, and the axioelectric cross section may be computed for arbitrary axion mass [21].

The expected event rate for an ALP absorption can be parameterized in terms of the axioelectric coupling  $g_{ae}$  and the axion mass  $m_a$ , and scales with the photoelectric cross section  $\sigma_{\text{p.e.}}$ :

$$R = \rho_{\text{DM}} \frac{3g_{ae}^2 c m_a}{16\pi\alpha m_e^2} \sigma_{\text{p.e.}}(m_a c^2) \quad (26)$$

To calculate the ALP signal spectrum in the quantized regime, the ionization model described in Sec. 2 is employed, and the quantized spectrum is again convolved with  $\sigma_{\langle E \rangle}$  with CT and II accounted for (see Sec. 2.2).

## 3.3 Limit Setting

The 90 % confidence level upper limit is calculated using a Poisson counting method. This method is applied without background subtraction and used a signal-only hypothesis. The Poisson upper limit is determined by first calculating the limit for each of the first six  $e^-h^+$ -pair peaks separately and then by selecting the

lowest limit at each DM mass. To account for the look-elsewhere effect, the confidence level of the Poisson upper limit for each individual  $e^-h^+$ -pair peak,  $C_{n_l}$  is determined by:

$$C_{n_l} = c^{\frac{1}{n_l}}, \quad (27)$$

where  $c = 0.9$  is the end result confidence level and  $n_l$  is the number of separate limits being compared. For example, if the limits from all six  $e^-h^+$ -pair peaks are being compared, each individual limit would be computed with a confidence level of 98.26%. The energy-dependent dark matter signal models at each DM mass,  $S_{\text{DM}}(E, m_{\text{DM}})$ , are computed initially with the arbitrary values of the effective mixing parameter  $\varepsilon_{\text{eff},0} = 5 \times 10^{-13}$ , the axioelectric coupling constant  $g_{ae,0} = 5 \times 10^{-11}$ , and the dark matter-electron cross section  $\bar{\sigma}_{e,0} = 10^{-37} \text{ cm}^2$  for dark photon absorption, axion-like particle absorption, and light dark matter electron scattering, respectively. The models are subsequently multiplied by the energy-dependent efficiency curve  $f(E)$  and the exposure  $X$ . To calculate the Poisson upper limit for an interval  $[E_1, E_2]$ , the  $C_{n_l}$  upper limit is computed on the number of observed events between  $E_1$  and  $E_2$ ,  $N_{\text{obs}}^{E_1 E_2}(C_{n_l})$ , and  $S_{\text{DM}}(E, m_{\text{DM}}) \times f(E) \times X$  is integrated between  $E_1$  and  $E_2$ . Using the relationships between the limit setting parameters and event rate discussed in Sections 3.2.1, 3.2.2, and 3.2.3, the Poisson upper limits at a given  $C_{n_l}$  and  $m_{\text{DM}}$  are given as:

$$\begin{aligned} \bar{\sigma}_e(m_\chi, C_{n_l}) &= \frac{N_{\text{obs}}^{E_1 E_2}(C_{n_l}) \cdot \bar{\sigma}_{e,0}}{X \int_{E_1}^{E_2} S_\chi(E, m_\chi) \times f(E) dE} \\ \varepsilon_{\text{eff}}(m_V, C_{n_l}) &= \sqrt{\frac{N_{\text{obs}}^{E_1 E_2}(C_{n_l}) \cdot \varepsilon_{\text{eff},0}^2}{X \int_{E_1}^{E_2} S_V(E, m_V) \times f(E) dE}} \\ g_{ae}(m_a, C_{n_l}) &= \sqrt{\frac{N_{\text{obs}}^{E_1 E_2}(C_{n_l}) \cdot g_{ae,0}^2}{X \int_{E_1}^{E_2} S_a(E, m_a) \times f(E) dE}} \end{aligned} \quad (28)$$

The interval  $[E_1, E_2]$  for each  $e^-h^+$ -pair peak is  $\pm 3\sigma_{\langle E \rangle}$  centered around each peak in the DM signal model, where  $\sigma_{\langle E \rangle}$  is the weighted average energy resolution described in Section 2. For dark photon and ALP absorption, the  $n^{\text{th}}$  peak location in the signal model is  $n \cdot e \cdot V_{\text{bias}} + m_{a/V} \cdot c^2$ , where  $m_{a/V}$  is either the dark photon or axion-like particle mass. For light dark matter electron scattering, the  $n^{\text{th}}$  peak location in the signal model is  $n \cdot e \cdot V_{\text{bias}} + \langle E_r \rangle$ , where  $\langle E_r \rangle$  is the average of the recoil energies weighted by their relative probability at the  $n^{\text{th}}$  peak for a given mass  $m_\chi$ .

The choice and number of  $e^-h^+$ -pair peak limits  $n_l$  to compare and select from depends on the dark matter mass. For instance, the limit calculated at the first  $e^-h^+$ -pair peak is typically never selected as the lowest limit at high dark matter masses. To avoid being overly conservative by comparing all six  $e^-h^+$ -pair peak limits at all masses, and to avoid biasing toward computing only 1  $e^-h^+$ -pair peak limit that is known to be the lowest at a given mass, a procedure was developed to determine the choice and number of  $e^-h^+$ -pair peak limits to select between by using the 10% of the DM-search data used in the initial stage of the blind analysis. The procedure works as follows for each dark matter mass:

1. Calculate the limit at each  $e^-h^+$ -pair peak using the initial-stage DM-search data and exposure at a 90% confidence level.
2. Calculate the limit at each  $e^-h^+$ -pair peak using the initial-stage DM-search data and exposure at a 90% confidence level again assuming:
  - (a) the number of observed events  $N_{\text{obs}}$  is a statistical under-fluctuation and is adjusted to  $N_{\text{obs}}^u$  such that  $N_{\text{obs}}^u - \sigma(N = N_{\text{obs}}^u) = N_{\text{obs}}$ ;
  - (b) the number of observed events  $N_{\text{obs}}$  is a statistical over-fluctuation and is adjusted to  $N_{\text{obs}}^o$  such that  $N_{\text{obs}}^o + \sigma(N = N_{\text{obs}}^o) = N_{\text{obs}}$ .
3. Calculate the limit at each  $e^-h^+$ -pair peak using the initial-stage DM-search data at a 90% confidence level after scaling the exposure and  $N_{\text{obs}}$  by a factor of 9 to estimate the results after unblinding the data.

4. Calculate the limit at each  $e^-h^+$ -pair peak using the initial-stage DM-search data at a 90 % confidence level after scaling the exposure and  $N_{\text{obs}}$  by a factor of 9 again assuming:
  - (a) the number of observed events  $9 \times N_{\text{obs}}$  is a statistical under-fluctuation and is adjusted to  $N_{\text{obs}}^u$  such that  $N_{\text{obs}}^u - \sigma(N = N_{\text{obs}}^u) = 9 \times N_{\text{obs}}$ ;
  - (b) the number of observed events  $9 \times N_{\text{obs}}$  is a statistical over-fluctuation and is adjusted to  $N_{\text{obs}}^o$  such that  $N_{\text{obs}}^o + \sigma(N = N_{\text{obs}}^o) = 9 \times N_{\text{obs}}$ .
5. Choose the limits corresponding to the  $e^-h^+$ -pair peaks that were selected as the lowest limit at any point during steps 1–4.

The term  $\sigma(N)$  shown in the procedure above is the standard deviation of observing  $N$  events assuming Poisson statistics. As the limits were calculated separately for each Fano factor assumption, this procedure was also followed separately for each Fano factor value. The choice and number of  $e^-h^+$ -pair peak limits are subsequently applied to the unblinded DM-search data to produce the final results, and are included in this data release in the files named `SupplData/limChoice_<DM model>-100V_F=<Fano factor>.tsv`. In these files, the first column is DM mass in units of  $\text{MeV}/c^2$  for light dark matter electron scattering and  $\text{keV}/c^2$  for dark photon and axion-like particle absorption. Columns 2–7 correspond to  $e^-h^+$ -pair peaks 1–6 and indicate whether or not they were used in the limit setting procedure (1 means it was used, 0 means it was not).

The final limit results and their propagated uncertainties are calculated for each Fano factor assumption ( $F = 0.155$ ,  $F = 10^{-4}$ , and  $F = 0.3$ ) separately. To quantify the impact of systematic uncertainties, the limits are recalculated 5000 times with random variates for the energy calibration, energy resolution, CT and II fractions, efficiency, and photoelectric absorption cross section according to their corresponding means and/or uncertainties. The following list describes the distributions used to draw the random variates:

- Energy Calibration: Gaussian distribution with a mean of 0 eV and a standard deviation of 0.5 eV. This is applied as a shift in the dark matter signal model and a shift in the limit setting window.
- Energy Resolution: Gaussian distribution with a mean of 3.6 eV and a standard deviation of 0.3 eV. This affects both the dark matter signal modal and the limit setting window size.
- Charge Trapping: Gaussian distribution with a mean of 0.11 and a standard deviation of 0.03. This affects the dark matter signal model. See Section 2 for more details.
- Impact Ionization: Gaussian distribution with a mean of 0.02 and a standard deviation of 0.03. The distribution is truncated at 0. This affects the dark matter signal model. See Section 2 for more details.
- Efficiency: Gaussian distribution with a mean of 0 and a standard deviation of 1. For a randomly chosen value of  $\sigma_f$ , the efficiency curve used will be  $f(E) = f_m(E) + \sigma_f f_u(E)$ , where  $f_m(E)$  and  $f_u(E)$  are the mean and uncertainty envelope of the efficiency curve, respectively. Due to the large uncertainty envelope in the efficiency curve, there are instances where  $f(E) > 1$ . Although this represents a non-physical situation, there is a well-understood linear relationship between the efficiency and the DM signal rates. The mean limit value is computed using the individual limits with all variates of  $\sigma_f$  even if  $f(E) > 1$ . However, the limit *uncertainty* is computed only with those limits with  $\sigma_f$  such that  $f(E) \leq 1$ . This ensures that the limit uncertainty is computed with only physically possible efficiencies. The efficiency curve is discussed in Section 1.1.2.
- Photoelectric Absorption Cross Section: Random choice between the upper, lower, and nominal photoelectric absorption cross section curves, where each choice has equal weight. Only applicable to the dark photon and axion-like particle absorption limits. See Section 1.2 for more details.

At each  $e^-h^+$ -pair peak, Fano factor  $F$ , and DM mass, the average of all 5000 limit calculations is computed, and the  $\pm 1\sigma$  equivalent values from the resulting limit distributions are used as the uncertainty on the limit. The  $\pm 1\sigma$  equivalent values correspond to the 15.9 % and 84.1 % points on each limit distribution's cumulative probability distribution function. The  $e^-h^+$ -pair peak with the lowest limit average among those that passed the selection criteria described above is selected, and its average and corresponding uncertainty

are used as the result at the given DM mass and Fano factor. The reported exclusion limits are those calculated using a Fano factor value of 0.155 in the ionization model at each DM mass. The reported limit uncertainties are the envelope of the  $\pm 1\sigma$  uncertainties determined from all three limits obtained using the different Fano factor assumptions at each DM mass.

## References

- [1] SuperCDMS Collaboration. Constraints on low-mass, relic dark matter candidates from a surface-operated supercdms single-charge sensitive detector. *Phys. Rev. D*, 102:091101, Nov 2020. doi: 10.1103/PhysRevD.102.091101. URL <https://link.aps.org/doi/10.1103/PhysRevD.102.091101>.
- [2] Y. Hochberg, T. Lin, and K. M. Zurek. Absorption of light dark matter in semiconductors. *Phys. Rev. D*, 95(2):023013, January 2017. doi: 10.1103/PhysRevD.95.023013.
- [3] K. Rajkanan, R. Singh, and J. Shewchun. Absorption coefficient of silicon for solar cell calculations. *Solid State Electron.*, 22:793, 1979. ISSN 0038-1101. doi: [https://doi.org/10.1016/0038-1101\(79\)90128-X](https://doi.org/10.1016/0038-1101(79)90128-X). URL <http://www.sciencedirect.com/science/article/pii/003811017990128X>.
- [4] SuperCDMS Collaboration. First Dark Matter Constraints from a SuperCDMS Single-Charge Sensitive Detector. *Phys. Rev. Lett.*, 121(5):051301, 2018. doi: 10.1103/PhysRevLett.122.069901,10.1103/PhysRevLett.121.051301. [Erratum: *Phys. Rev. Lett.*122,no.6,069901(2019)].
- [5] A. Aguilar-Arevalo, D. Amidei, D. Baxter, G. Canelo, B. A. Cervantes Vergara, A. E. Chavarria, E. Darragh-Ford, J. R. T. de Mello Neto, J. C. D’Olive, J. Estrada, et al. Constraints on Light Dark Matter Particles Interacting with Electrons from DAMIC at SNOLAB. *Phys. Rev. Lett.*, 123:181802, 2019. doi: 10.1103/PhysRevLett.123.181802. URL <https://link.aps.org/doi/10.1103/PhysRevLett.123.181802>.
- [6] O. Abramoff, L. Barak, I. M. Bloch, L. Chaplinsky, M. Crisler, Dawa, A. Drlica-Wagner, R. Essig, J. Estrada, E. Etzion, et al. Sensei: Direct-detection constraints on sub-gev dark matter from a shallow underground run using a prototype skipper ccd. *Phys. Rev. Lett.*, 122:161801, 2019. doi: 10.1103/PhysRevLett.122.161801. URL <https://link.aps.org/doi/10.1103/PhysRevLett.122.161801>.
- [7] R. Essig, A. Manalaysay, J. Mardon, P. Sorensen, and T. Volansky. First direct detection limits on sub-gev dark matter from xenon10. *Phys. Rev. Lett.*, 109:021301, 2012. doi: 10.1103/PhysRevLett.109.021301. URL <https://link.aps.org/doi/10.1103/PhysRevLett.109.021301>.
- [8] R. Essig, T. Volansky, and T.-T. Yu. New constraints and prospects for sub-gev dark matter scattering off electrons in xenon. *Phys. Rev. D*, 96:043017, 2017. doi: 10.1103/PhysRevD.96.043017. URL <https://link.aps.org/doi/10.1103/PhysRevD.96.043017>.
- [9] E. Aprile, J. Aalbers, F. Agostini, M. Alfonsi, L. Althueser, F. D. Amaro, M. Anthony, F. Arneodo, L. Baudis, B. Bauermeister, et al. Dark Matter Search Results from a One Ton-Year Exposure of XENON1T. *Phys. Rev. Lett.*, 121:111302, 2018. ISSN 1079-7114. doi: 10.1103/physrevlett.121.111302. URL <http://dx.doi.org/10.1103/PhysRevLett.121.111302>.
- [10] I. M. Bloch, R. Essig, K. Tobioka, T. Volansky, and T.-T. Yu. Searching for dark absorption with direct detection experiments. *J. High Energy Phys.*, 2017:1029, 2017. doi: 10.1007/JHEP06(2017)087. URL [https://doi.org/10.1007/JHEP06\(2017\)087](https://doi.org/10.1007/JHEP06(2017)087).
- [11] T. Aralis, T. Aramaki, I. J. Arnquist, E. Azadbakht, W. Baker, S. Banik, D. Barker, C. Bathurst, D. A. Bauer, L. V. S. Bezerra, et al. Constraints on dark photons and axionlike particles from the SuperCDMS Soudan experiment. *Phys. Rev. D*, 101:052008, 2020. doi: 10.1103/PhysRevD.101.052008. URL <https://link.aps.org/doi/10.1103/PhysRevD.101.052008>.
- [12] H. An, M. Pospelov, J. Pradler, and A. Ritz. Direct detection constraints on dark photon dark matter. *Phys. Lett. B*, 747:331, 2015. ISSN 0370-2693. doi: <https://doi.org/10.1016/j.physletb.2015.06.018>. URL <http://www.sciencedirect.com/science/article/pii/S0370269315004402>.

- [13] N. Viaux, M. Catelan, P. B. Stetson, G. G. Raffelt, J. Redondo, A. A. R. Valcarce, and A. Weiss. Neutrino and axion bounds from the globular cluster m5 (ngc 5904). *Phys. Rev. Lett.*, 111:231301, 2013. doi: 10.1103/PhysRevLett.111.231301. URL <https://link.aps.org/doi/10.1103/PhysRevLett.111.231301>.
- [14] M. M. M. Bertolami, B. E. Melendez, L. G. Althaus, and J. Isern. Revisiting the axion bounds from the Galactic white dwarf luminosity function. *J. Cosmol. Astropart. Phys.*, 1410:069, 2014. doi: 10.1088/1475-7516/2014/10/069.
- [15] M. Tanabashi, K. Hagiwara, K. Hikasa, K. Nakamura, Y. Sumino, F. Takahashi, J. Tanaka, K. Agashe, G. Aielli, C. Amsler, et al. Review of Particle Physics. *Phys. Rev. D*, 98:030001, 2018. doi: 10.1103/PhysRevD.98.030001. URL <https://link.aps.org/doi/10.1103/PhysRevD.98.030001>.
- [16] V S Vavilov. Radiation ionization processes in germanium and silicon crystals. *Soviet Physics Uspekhi*, 4(5):761, 1962. URL <http://stacks.iop.org/0038-5670/4/i=5/a=A12>.
- [17] K. Ramanathan and N. Kurinsky. Ionization yield in silicon for ev-scale electron-recoil processes. *Phys. Rev. D*, 102:063026, Sep 2020. doi: 10.1103/PhysRevD.102.063026. URL <https://link.aps.org/doi/10.1103/PhysRevD.102.063026>.
- [18] Yonit Hochberg, Tongyan Lin, and Kathryn M. Zurek. Absorption of light dark matter in semiconductors. *Phys. Rev. D*, 95:023013, Jan 2017. doi: 10.1103/PhysRevD.95.023013. URL <https://link.aps.org/doi/10.1103/PhysRevD.95.023013>.
- [19] PandaX-II Collaboration. Limits on axion couplings from the first 80 days of data of the pandax-ii experiment. *Phys. Rev. Lett.*, 119:181806, Nov 2017. doi: 10.1103/PhysRevLett.119.181806. URL <https://link.aps.org/doi/10.1103/PhysRevLett.119.181806>.
- [20] Roberto D. Peccei. *The Strong CP Problem and Axions*, pages 3–17. Springer Berlin Heidelberg, Berlin, Heidelberg, 2008. ISBN 978-3-540-73518-2. doi: 10.1007/978-3-540-73518-2\_1. URL [https://doi.org/10.1007/978-3-540-73518-2\\_1](https://doi.org/10.1007/978-3-540-73518-2_1).
- [21] A. Derevianko, V. A. Dzuba, V. V. Flambaum, and M. Pospelov. Axio-electric effect. *Phys. Rev. D*, 82:065006, Sep 2010. doi: 10.1103/PhysRevD.82.065006. URL <https://link.aps.org/doi/10.1103/PhysRevD.82.065006>.
